# Supplementary material for: Private Webmail 2.0: Simple and Easy-to-Use Secure Email
Source: arXiv:1510.08435 source file (2016-08-09)
Supplement: Supplementary file 1 [file appendix.tex]

\setcounter{figure}{0}
\setcounter{table}{0}
\appendix

\section{Pwm User Study}

\subsection{Introduction}
\label{appx:intro}

\textit{At the beginning of each user study the following was read to the participant by the study coordinator.}\newline

Welcome to our Gmail study. I am the study coordinator and am here to assist you as needed.

In this study, you will be using Gmail to complete several scenarios. In each scenario you will play the role of another person. I will provide you with information about this person. During the scenarios, please use this provided information and not your own personal information. Please protect any sensitive information for this person just as if it was your own.

During the course of the study we will record what is happening on your screen. This video will not be seen by anyone besides the researchers and will be destroyed once our research is complete. We will not collect any personally identifying information.  Any data, besides the screen recording and answers to the study survey, will be deleted automatically upon your completion of the study.

You will receive \$10.00 as compensation for your participation in this study. The expected time commitment is approximately 30 minutes. If you have any questions or concerns, feel free to ask me. You can end participation in this survey at any time and we will delete all data collected at your request. 

You may now proceed with the survey on the left-most computer. I will remain in the room to observe the study and also to answer any questions you may have.

\subsection{Scenarios}
\label{appx:scenarios}

\textit{These were the two scenarios used in the study. The first scenario covers Task 1 -- Task 4 and the second scenario covers Task 5 and Task 6.}

\subsubsection{Scenario 1}

In this scenario, you have applied for a job with National Citadel. Last weekend they flew you out for a final interview. They told you they would email you instructions for getting your expenses reimbursed.

All information you will need to complete this scenario is provided below.

During this scenario you will receive and respond to several emails. Until you receive an email with a confirmation code, please continue to check your inbox for new email messages. Be aware that sometimes there will be a slight delay (30-60 seconds) before you receive an email.

At this time, please log into your email account where you should see an email message from National Citadel. If you don't see such a message, ask the study coordinator for help.

\begin{center}
\vspace{6pt}
\textbf{\large Scenario 1 Persona}
\vspace{3pt}

\begin{tabular}{|l|l|}
	\toprule

	Social Security Number & 834-23-1339 \\ \midrule
	State of residence & [redacted] \\ \midrule
	Date of birth & February 20, 1988 \\ \midrule
	Bank account number & 2365-9814-4907 \\ \midrule
	Bank routing number & 097-154-228 \\
	\bottomrule
\end{tabular}
\end{center}

\vspace{\baselineskip}
\subsubsection{Scenario 2}

In this scenario, you have received a text message from your spouse (spouse@[redacted]) asking for help logging in to your credit card website. Your spouse has asked you to email him/her the account username and password.

This information is sensitive, so you want to encrypt it. You know that your spouse has never used encrypted email before. Please do whatever you think you would do in real life to send them this information encrypted with Pwm.

All information you will need to complete this scenario is provided below.

During this scenario you will receive and respond to several emails. Until you receive an email with a confirmation code, please continue to check your inbox for new email messages. Be aware that sometimes there will be a slight delay (30-60 seconds) before you receive an email.

\begin{center}
\vspace{6pt}
\textbf{\large Scenario 2 Persona}
\vspace{3pt}

\begin{tabular}{|l|l|}
	\toprule

	Account username & family343 \\ \midrule
	Account password & b@nkp@ssword \\ \midrule
	Credit card number & 4716-9364-5318-3222 \\ \midrule
	Credit card CCV & 992 \\
	\bottomrule
\end{tabular}
\end{center}

\vspace{\baselineskip}
\subsection{Task Emails}
\label{appx:emails}

\subsubsection{Task 1}

\vspace{6pt}
\noindent\textit{Initial email.}\\
\textbf{Encrypted}: Yes \\
\textbf{From}: finances@nationalcitadel.com \\
\textbf{Subject}: Receipt Reimbursement \\
\textbf{Greeting}: Hi [participant's name], thank you for interviewing with National Citadel this week. In order to process your expense reimbursement, please reply to this email with your Social Security Number and a picture of your receipts for your purchases. Company policy requires that you send us this information encrypted. We use Pwm to encrypt email. This email includes directions for setting up Pwm. After setting up Pwm, you will be able to encrypt the required information. Thanks, --Jen Cobb\\
\textbf{Encrypted Body}: Now that you are running Pwm, you can simply reply to this message, and your information will automatically be encrypted.

\vspace{6pt}
\noindent\textit{If the participant encrypts the requested data.}\\
\textbf{Encrypted}: No \\
\textbf{From}: emailstudy@[redacted] \\
\textbf{Subject}: Task Complete \\
\textbf{Body}: Hi [participant's name], congratulations on completing your first task. Please continue to watch your inbox for more communications from National Citadel. --ISRL Research

\vspace{6pt}
\noindent\textit{If the participants does not encrypt the requested data.}\\
\textbf{Encrypted}: No \\
\textbf{From}: finances@nationalcitadel.com \\
\textbf{Subject}: Re: Receipt Reimbursement \\
\textbf{Body}: Hi [participant's name], it looks like you didn't send those details securely. Please resend with encryption enabled. Thanks, --Jen Cobb

\subsubsection{Task 2}

\vspace{6pt}
\noindent\textit{Participants instructed to close browser and then reopen Gmail.}\\
\textbf{Encrypted}: No \\
\textbf{From}: emailstudy@[redacted] \\
\textbf{Subject}: Scenario Instructions \\
\textbf{Body}: Before we proceed with the scenario, please close Chrome. This simulates time passing after your interview.
After Chrome is shut down, you may re-open Chrome and navigate to Gmail. Thanks, --ISRL Research

\vspace{6pt}
\noindent\textit{Initial email.}\\
\textbf{Encrypted}: Yes \\
\textbf{From}: hiring@nationalcitadel.com \\
\textbf{Subject}: National Citadel Offer \\
\textbf{Greeting}: This encrypted email contains details about your employment offer with National Citadel. Please decrypt to view.\\
\textbf{Encrypted Body}: Congratulations [participant's name]! We were very impressed with your performance in the interviews and are excited to extend a full-time offer. See below for the details. Please look over the offer and, if it is acceptable, reply to us so we can proceed with the hiring. 
Also, please CC your acceptance to your manager, Kaylee Clark, at kclark@nationalcitadel.com.
We look forward to your reply. Regards,
--Rory Tam

\begin{center}
\includegraphics[height=0.57\textheight]{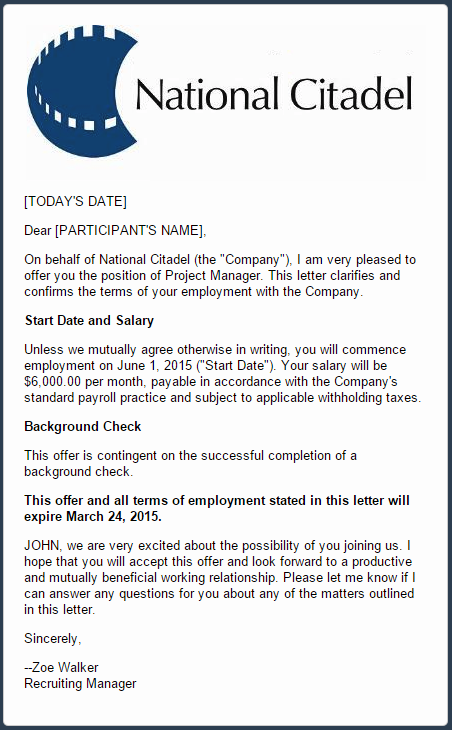}
\end{center}

\vspace{6pt}
\noindent\textit{If the participant encrypts the requested data.}\\
\textbf{Encrypted}: Yes \\
\textbf{From}: hiring@nationalcitadel.com \\
\textbf{Subject}: Re: National Citadel Offer \\
\textbf{Encrypted Body}: Hi [participant's name], we received your acceptance and are excited to begin the hiring process. As part of the onboarding procedure, you will be receiving emails from our Background Check and Payroll departments. Please reply to these emails with the requested information, so we can proceed with your hire.
Congratulations once again on joining our team. Regards,
--Rory Tam

\vspace{6pt}
\noindent\textit{If the participants does not CC Kaylee Clark.}\\
\textbf{Encrypted}: Yes \\
\textbf{From}: hiring@nationalcitadel.com \\
\textbf{Subject}: Re: National Citadel Offer \\
\textbf{Encrypted Body}: Hi [participant's name], it looks like you didn't CC your acceptance to your manager, Kaylee Clark, at kclark@nationalcitadel.com. Please resend your acceptance and be sure to CC her.
Thanks,
--Rory Tam

\vspace{6pt}
\noindent\textit{If the participants does not encrypt the requested data.}\\
\textbf{Encrypted}: Yes \\
\textbf{From}: hiring@nationalcitadel.com \\
\textbf{Subject}: Re: National Citadel Offer \\
\textbf{Greeting}: There was a problem with your reply. Please decrypt this message to view.\\
\textbf{Encrypted Body}: Hi [participant's name], it looks like you didn't encrypt your response. Please resend your acceptance and be sure to encrypt it.
Thanks,
--Rory Tam

\vspace{6pt}
\noindent\textit{If the participants does not CC Kaylee Clark and does not encrypt the requested data.}\\
\textbf{Encrypted}: Yes \\
\textbf{From}: hiring@nationalcitadel.com \\
\textbf{Subject}: Re: National Citadel Offer \\
\textbf{Greeting}: There was a problem with your reply. Please decrypt this message to view.\\
\textbf{Encrypted Body}: Hi [participant's name], it looks like you didn't CC your acceptance to your manager, Kaylee Clark, at kclark@nationalcitadel.com. Also, you seem to have sent your reply insecurely. Please resend your acceptance; be sure to CC her, and be sure to use encryption.
Thanks,
--Rory Tam

\subsubsection{Task 3}

\vspace{6pt}
\noindent\textit{Initial email.}\\
\textbf{Encrypted}: No \\
\textbf{From}: hiring@nationalcitadel.com \\
\textbf{Subject}: National Citadel Background Check \\
\textbf{Body}: Hello [participant's name], we have received your hiring details and are proceeding with a background check. Please fill out the following details and forward them to our Background Check provider, backgroundcheck@[redacted]. As a reminder, please encrypt all sensitive communications with other entities regarding your employment with National Citadel.\\
- Full name\\
- Date of birth\\
- Social Security Number\\
- State of residence\\
Thanks,
--Simon Turner

\vspace{6pt}
\noindent\textit{If the participant encrypts the requested data.}\\
\textbf{Encrypted}: Yes \\
\textbf{From}: backgroundcheck@[redacted] \\
\textbf{Subject}: Re: Fwd: National Citadel Background Check \\
\textbf{Encrypted Body}: Hi [participant's name], thanks for forwarding your background check details. We'll get started right away. National Citadel will inform you when your check is complete.
Regards,
--Inara Sanchez

\vspace{6pt}
\noindent\textit{If the participants does not encrypt the requested data.}\\
\textbf{Encrypted}: Yes \\
\textbf{From}: backgroundcheck@[redacted] \\
\textbf{Subject}: Re: Fwd: National Citadel Background Check \\
\textbf{Greeting}: Hi [participant's name], it looks like you sent us these background check details insecurely. Please re-forward with encryption enabled.
Thanks,
--Inara Sanchez

\vspace{6pt}
\noindent\textit{If the participants replies instead of sending the data to the background check company.}\\
\textbf{Encrypted}: No \\
\textbf{From}: hiring@nationalcitadel.com \\
\textbf{Subject}: Re: National Citadel Background Check \\
\textbf{Body}: Hi [participant's name], it looks like you replied to us instead of forwarding your details to our background check provider. Please forward to backgroundcheck@[redacted].
Thanks,
--Inara Sanchez

\subsubsection{Task 4}

\vspace{6pt}
\noindent\textit{Initial email.}\\
\textbf{Encrypted}: No \\
\textbf{From}: payroll@nationalcitadel.com \\
\textbf{Subject}: National Citadel Direct Deposit Information \\
\textbf{Body}: Hi [participant's name], we are proceeding with your hire and need your direct deposit information. Please reply to this email with your bank account number and routing number so that we can ensure your paychecks are properly deposited.
Thanks,
--Matthew Reynolds

\vspace{6pt}
\noindent\textit{Upon participants sending the requested data.}\\
\textbf{Encrypted}: No \\
\textbf{From}: emailstudy@[redacted] \\
\textbf{Subject}: Re: Fwd: Task Complete \\
\textbf{Body}: Hi [participant's name], you have completed this scenario. Please return to Qualtrics and enter your confirmation code.
Confirmation code: 1071
Thanks,
--ISRL Research

\subsubsection{Task 5}

\vspace{6pt}
\noindent\textit{If the participant encrypts the requested data.}\\
Continue to Task 6.

\vspace{6pt}
\noindent\textit{If the participants does not encrypt the requested data.}\\
\textbf{Encrypted}: No \\
\textbf{From}: emailstudy@[redacted] \\
\textbf{Subject}: Task Incomplete \\
\textbf{Body}: Hi [participant's name], please try again to send the credit card details securely. It looks like the message you just sent was unencrypted.
Thanks,
--ISRL Research

\subsubsection{Task 6}

\vspace{6pt}
\noindent\textit{Initial email.}\\
\textbf{Encrypted}: No \\
\textbf{From}: spouse@[redacted] \\
\textbf{Subject}: Re: Credit card details \\
\textbf{Body}: Hi, thanks for the login details. Now it's saying I need the last four digits of the credit card, and the CCV number. Can you send those to me?
Thanks

\vspace{6pt}
\noindent\textit{Upon participants sending the requested data.}\\
\textbf{Encrypted}: No \\
\textbf{From}: emailstudy@[redacted] \\
\textbf{Subject}: Re: Fwd: Task Complete \\
\textbf{Body}: Hi [participant's name], you have completed this scenario. Please return to Qualtrics and enter your confirmation code.
Confirmation code: 8472
Thanks,
--ISRL Research

\section{Questionnaires}

\subsection{Demographic Questionnaire}
\label{appx:demographic}

\noindent \textbf{What is your gender?} \textit{Male, Female}\\

\noindent \textbf{What is your age?}\\
\textit{
\vspace{-10pt}
\begin{itemize}[label=$\cdot$,leftmargin=10pt,noitemsep,nolistsep]
\item 18 -- 24 years old
\item 25 -- 34 years old
\item 35 -- 44 years old
\item 45 -- 54 years old
\item 55 years or older\\
\end{itemize}
}

\noindent \textbf{What is the highest degree or level of school you have completed?}
\textit{
\begin{itemize}[label=$\cdot$,leftmargin=10pt,noitemsep,nolistsep]
\item Some school, no high school diploma
\item High school graduate, diploma or the equivalent (for example: GED)
\item Some college or university credit, no degree
\item College or university degree
\item Graduate or professional degree\\
\end{itemize}
}

\noindent \textbf{What is your occupation or major?}\\

\noindent \textbf{How often do you use Gmail through your browser?}
\textit{
\begin{itemize}[label=$\cdot$,leftmargin=10pt,noitemsep,nolistsep]
\item Less than Once a Month
\item Once a Month
\item 2 -- 3 Times a Month
\item Once a Week
\item 2 -- 3 Times a Week
\item Once a Day
\item Many Times a Day\\
\end{itemize}
}

\subsection{Study Questionnaire}
\label{appx:questionnaire}

\noindent You have completed all of the scenarios. You will now be asked several questions concerning your experience with Pwm.\\

\noindent \textbf{Please answer the following question about Pwm. Try to give your immediate reaction to each statement without pausing to think for a long time. Mark the middle column if you don't have a response to a particular statement.}\\
\textit{Strongly Disagree, Disagree, Neither Agree nor Disagree, Agree, Strongly Agree}
\begin{itemize}[label=$\Bigcdot$]
	\item I think that I would like to use this system frequently.
	\item I found the system unnecessarily complex.
	\item I thought the system was easy to use.
	\item I think that I would need the support of a technical person to be able to use this system.
	\item I found the various functions in this system were well integrated.
	\item I thought there was too much inconsistency in this system.
	\item I would imagine that most people would learn to use this system very quickly.
	\item I found the system very cumbersome to use.
	\item I felt very confident using the system.
	\item I needed to learn a lot of things before I could get going with this system.\\
\end{itemize}

\noindent \textbf{Please answer the following questions about Pwm. Try to give your immediate reaction to each statement without pausing to think for a long time. Mark the middle column if you don't have a response to a particular statement.}\\
\textit{Strongly Disagree, Disagree, Neither Agree nor Disagree, Agree, Strongly Agree}
\begin{itemize}[label=$\Bigcdot$]
	\item I want to be able to encrypt all of my email.
	\item I want to be able to encrypt sensitive email.
	\item I want to start using Pwm.
	\item I would use Pwm with my friends and family.
	\item My friends and family could easily start using Pwm.
	\item Pwm protects my email.\\
\end{itemize}

\noindent \textbf{What did you like most about using Pwm?}\\

\noindent \textbf{What would you change about Pwm?}\\

\noindent \textbf{Is there anything else you think that Pwm could do to be more useful for you personally?}\\

\noindent \textbf{If I encrypt an email using Pwm, who is able to read it?}\\
\textsc{Multiple selections allowed}
\textit{
\begin{itemize}[label=$\cdot$,leftmargin=10pt,noitemsep,nolistsep]
\item Me
\item The recipients
\item Gmail
\item Hackers who steal the email during transmission
\item Hackers who break into my account
\item Government Agencies, for example the NSA
\item Unsure\\
\end{itemize}}

\noindent \textbf{Can an email encrypted with Pwm have a fake "from" address?}\\
\textit{Yes, No. It depends, Unsure}\\

\noindent \textbf{Can an email encrypted with Pwm be modified by a third party (for example, Google or a hacker)?}\\
\textit{Yes, No. It depends, Unsure}\\

\noindent \noindent \textbf{Do you ever send sensitive information through email?}\\
\textit{Yes, No}\\

\noindent \texttt{Only seen if selected "Yes" to sending sensitive information through email.}\\
\noindent \textbf{What type of sensitive information do you send through email?}\\

\noindent \texttt{Only seen if selected "Yes" to sending sensitive information through email.}\\
\noindent \textbf{How often do you send sensitive information through email?}
\textit{
\begin{itemize}[label=$\cdot$,leftmargin=10pt,noitemsep,nolistsep]
\item Less than Once a Month
\item Once a Month
\item 2 -- 3 Times a Month
\item Once a Week
\item 2 -- 3 Times a Week
\item Once a Day
\item Many Times a Day\\
\end{itemize}
}

\noindent \textbf{What method do you prefer to use to send sensitive information?}\\
\textsc{Multiple selections allowed}\\
\textit{Email, Phone call, Text message, Fax, In person, Other}\\

\noindent \textbf{Prior to this study, had you ever encrypted your email before?}\\
\textit{Yes, No}\\

\noindent \texttt{Only seen if selected "Yes" to having previously used email encryption.}\\
\noindent \textbf{What software have you used to encrypt your email?}\\

\noindent \texttt{Only seen if selected "Yes" to having previously used email encryption.}\\
\noindent \textbf{Why did you need to encrypt your email?}\\

\noindent \textbf{If easy-to-use email encryption was available, would you be more likely to send sensitive information over email?}\\
\textit{Yes, No, It depends, Unsure}\\

\noindent \textbf{There are many ways to implement encrypted email. One approach is to tightly integrate with existing systems. For example, Pwm appears in the same page as Gmail. Another approach is to create a separate interface where you encrypt messages, and then copy these encrypted emails into your email client.The following are a list of possible approaches to encrypted email. Please rank them according to which you would prefer to use. (Higher is better, drag and drop to arrange).}
\\ \textsc{Initial ordering of options randomized.}
\textit{
\begin{itemize}[label=$\cdot$,leftmargin=10pt]
	\item Integrated tightly into a web-based email system.
	\item Integrated tightly into a desktop/mobile application.
	\item A desktop/mobile application that has a separate interface for encrypting messages.
	\item A browser extension that has a separate interface for encrypting messages.
	\item A web page that has a separate interface for encrypting messages.
	\item A email provider that only supports encrypted email.\\
\end{itemize}
}

\noindent \textbf{Please explain why you prefer your top ranked option.}\\

\noindent \textbf{Would you be willing to pay for a system that encrypts email?}\\
\textit{Yes, No, It depends, Unsure}\\

\noindent \texttt{Only seen if did not select "No" to whether willing to pay for email encryption.}\\
\noindent \textbf{How much money would you be willing to pay a month to encrypt your email?}\\

\onecolumn
\clearpage
\section{User Study Poster}
\label{appx:poster}

Recruitment poster used during study.

\vspace{12pt}
\begin{center}
\includegraphics[height=.90\textheight]{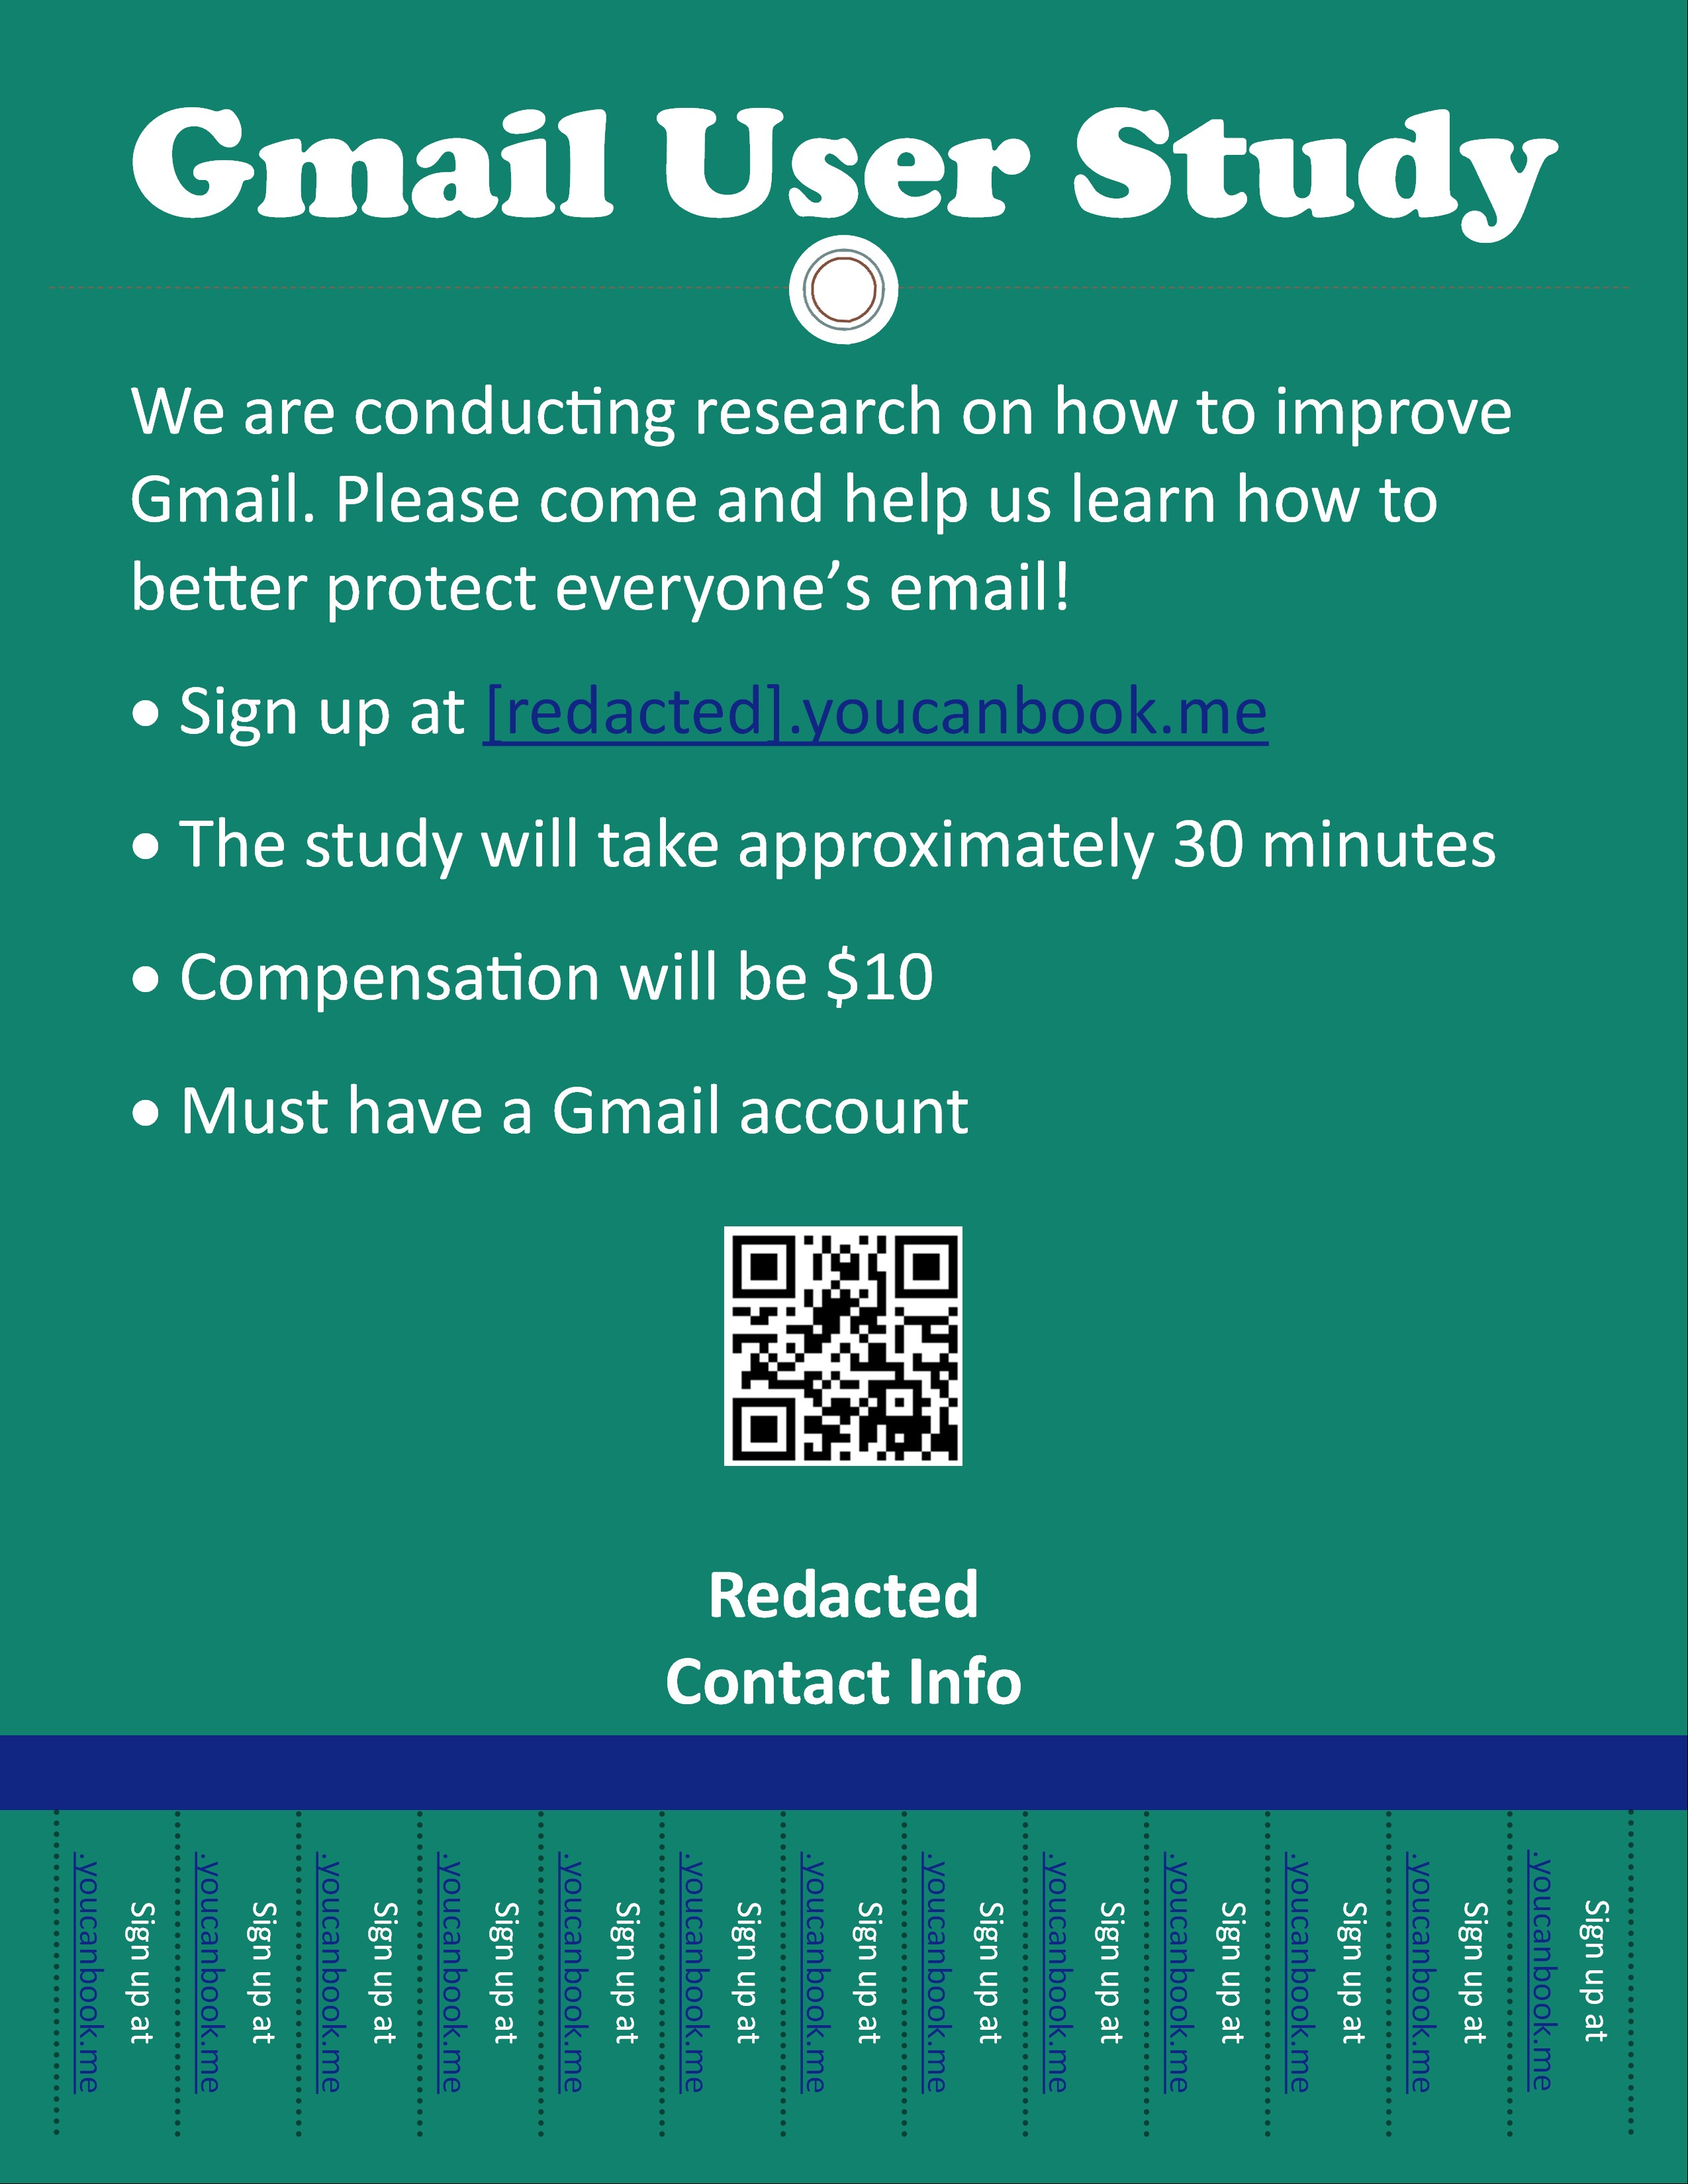}
\end{center}

\clearpage
\section{PWM Instructions}
\label{appx:pwminstructions}

Instructions for installing Pwm included with all email encrypted by Pwm. These instructions are hidden once participants are running Pwm.

\vspace{12pt}
\begin{center}
\includegraphics{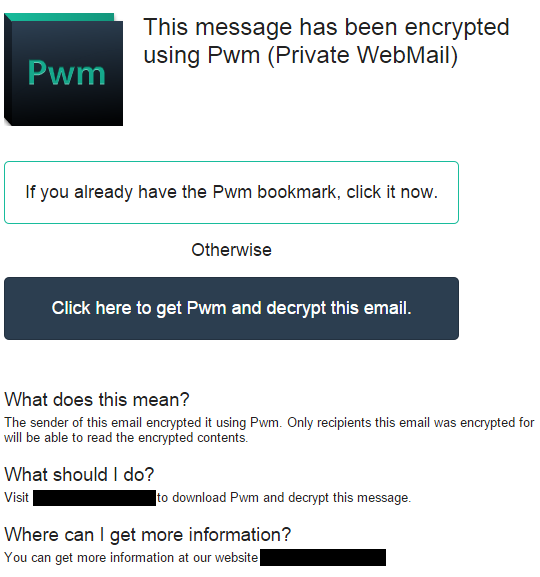}
\end{center}
